# Supplementary material for: Channel Tracking for Wireless Energy Transfer: A Deep Recurrent Neural Network Approach
Source: arXiv:1812.02986 source file (2018-12-07)
Supplement: Supplementary file 1 [file appendix.tex]

\appendices

\numberwithin{equation}{section}

\section*{Appendix A: Proof of Theorem \ref{thm_1}}

Let us define $ q_{k,n} = \sum_{i=n}^{N_{k}} p_{k,i} $, $\forall n,k$. Then the rate of (\ref{R_sum}) can be written as $ R_{k,n} ( \cdot ) =  \log_{2} \Big(  1 +  \frac{ h_{k,n} p_{k,n} }{ h_{k,n} \sum_{i=n+1}^{N_{k}} p_{k,i}  + \sigma^{2} }  \Big) = \log_{2} \Big(  \frac{ h_{k,n} q_{k,n} + \sigma^{2} }{ h_{k,n} q_{k,n+1}  + \sigma^{2} }  \Big)$, $1 \leq n < N_{k}$
and $ R_{k,N_{k}} ( \cdot ) =  \log_{2} \Big(  1 +  \frac{ h_{k,N_{k}} p_{k,N_{k}} }{  \sigma^{2} }  \Big) = \log_{2} \Big(  \frac{ h_{k,N_{k}} q_{k,N_{k}} + \sigma^{2} }{ \sigma^{2} }  \Big)$, $\forall k$.
From this, the objective function in (\ref{P1_obj}) can be written as (\ref{P1_2_obj}),
and the rate constraints in (\ref{P1_const_1}) can be written as (\ref{P1_2_const_1}) and (\ref{P1_2_const_2}).
Also, the power constraints in (\ref{P1_const_2}) can be written as (\ref{P1_2_const_3}) and (\ref{P1_2_const_4}).
Thus, with given $\{ \mathcal{N}_{k} \}$ and $\mathbf{W}$, (P1) can be recast into (P3).
Since the objective function in (\ref{P1_2_obj}) is concave and the constraints in (\ref{P1_2_const_1}) and (\ref{P1_2_const_2}) are linear, (P3) is a convex problem.

\section*{Appendix B: Proof of Theorem \ref{thm_2}}

The objective function of (P3) is increasing in $q_{k,n}$, $1 < n \leq N_{k}$, $\forall k$.
Thus, from the constraints in (\ref{P1_2_const_1}), we have $ q_{k,n+1} = \frac{ q_{k,n} }{ \gamma_{k,n} } - \frac{  (\gamma_{k,n} - 1) \sigma^{2}  }{  \gamma_{k,n} h_{k,n}  } $, $1 \leq n < N_{k}$, $\forall k$.
By recursion, we have the result of (\ref{power_allocation_2}).
Substituting (\ref{power_allocation_2}) into (P3), the optimization becomes: $ \underset{ \{  q_{k,1} \} }{\max}  \quad  \sum_{k=1}^{K} \log_{2} \Big( 1 +  \frac{ h_{k,1} q_{k,1} }{\sigma^{2}}  \Big) ~ {\rm s.t.} ~ q_{k,1} \geq  \psi_{k,N_{k}},  ~ \forall k, ~ \sum_{k=1}^{K} q_{k,1}  \leq  P$.
The solution to this problem can be obtained by using the Lagrange method as in (\ref{power_allocation}).
